# Supplementary material for: HEALTH-PARIKSHA: Assessing RAG Models for Health Chatbots in Real-World Multilingual Settings
Source: arXiv:2410.13671 source file (2025-12-01)
Supplement: Supplementary file 1 [file pa_scores.tex]

\section{LLM-evaluator scores for non-English languages}
\label{sec:llm-non-english}

\begin{table*}[h]
\small
\centering
\begin{tabular}{@{}lc|cccc@{}}
\toprule
\textbf{Model} & \textbf{AGG} & \textbf{COH} & \textbf{CON} & \textbf{FC} & \textbf{SS} \\ \midrule
\textsc{Qwen2.5-72B-Instruct} & 1.29 & 1.87 & 1.96 & 1.35 & 1.22 \\
\textsc{gpt-4} & 1.18 & 1.78 & 1.96 & 1.30 & 0.91 \\
\textsc{Mistral-Large-Instruct-2407} & 1.09 & 1.39 & 1.96 & 1.22 & 0.96 \\
\textsc{gemma-2-27b-it} & 0.92 & 1.30 & 1.91 & 1.04 & 0.65 \\
\textsc{gpt-4o} & 0.88 & 0.96 & 2.00 & 1.00 & 0.74 \\
\textsc{AryaBhatta-GemmaOrca-Merged} & 0.51 & 0.57 & 1.13 & 0.52 & 0.52 \\
\textsc{Meta-Llama-3.1-70B-Instruct} & 0.48 & 0.43 & 0.78 & 0.57 & 0.48 \\
\textsc{Kan-Llama-7B-SFT-v0.5} & 0.47 & 0.52 & 1.04 & 0.48 & 0.48 \\
\textsc{llama38bGenZ\_Vikas-Merged} & 0.47 & 0.52 & 1.00 & 0.43 & 0.57 \\
\textsc{Indic-gemma-7b-finetuned-sft-Navarasa-2.0} & 0.24 & 0.35 & 0.39 & 0.26 & 0.22 \\
\textsc{Phi-3.5-MoE-instruct} & 0.20 & 0.26 & 1.22 & 0.17 & 0.09 \\
\textsc{AryaBhatta-GemmaUltra-Merged} & 0.13 & 0.17 & 0.70 & 0.09 & 0.13 \\
\textsc{Ambari-7B-Instruct-v0.2} & 0.05 & 0.04 & 0.13 & 0.04 & 0.09 \\ \bottomrule
\end{tabular}
\caption{Metric-wise scores for Kannada}
\label{tab:kan-scores}
\end{table*}

\begin{table*}[h]
\small
\centering 
\begin{tabular}{@{}lc|cccc@{}}
\toprule
\textbf{Model} & \textbf{AGG} & \textbf{COH} & \textbf{CON} & \textbf{FC} & \textbf{SS} \\ \midrule
\textsc{Qwen2.5-72B-Instruct} & 1.29 & 1.87 & 1.96 & 1.35 & 1.22 \\
\textsc{gpt-4} & 1.18 & 1.78 & 1.96 & 1.30 & 0.91 \\
\textsc{Mistral-Large-Instruct-2407} & 1.09 & 1.39 & 1.96 & 1.22 & 0.96 \\
\textsc{gemma-2-27b-it} & 0.92 & 1.30 & 1.91 & 1.04 & 0.65 \\
\textsc{gpt-4o} & 0.88 & 0.96 & 2.00 & 1.00 & 0.74 \\
\textsc{AryaBhatta-GemmaOrca-Merged} & 0.51 & 0.57 & 1.13 & 0.52 & 0.52 \\
\textsc{Meta-Llama-3.1-70B-Instruct} & 0.48 & 0.43 & 0.78 & 0.57 & 0.48 \\
\textsc{Kan-Llama-7B-SFT-v0.5} & 0.47 & 0.52 & 1.04 & 0.48 & 0.48 \\
\textsc{llama38bGenZ\_Vikas-Merged} & 0.47 & 0.52 & 1.00 & 0.43 & 0.57 \\
\textsc{Indic-gemma-7b-finetuned-sft-Navarasa-2.0} & 0.24 & 0.35 & 0.39 & 0.26 & 0.22 \\
\textsc{Phi-3.5-MoE-instruct} & 0.20 & 0.26 & 1.22 & 0.17 & 0.09 \\
\textsc{AryaBhatta-GemmaUltra-Merged} & 0.13 & 0.17 & 0.70 & 0.09 & 0.13 \\
\textsc{Ambari-7B-Instruct-v0.2} & 0.05 & 0.04 & 0.13 & 0.04 & 0.09 \\ \bottomrule
\end{tabular}
\caption{Metric-wise scores for Tamil}
\label{tab:tam-scores}
\end{table*}

\begin{table*}[h]
\small
\centering 
\begin{tabular}{@{}lc|cccc@{}}
\toprule
\textbf{Model} & \textbf{AGG} & \textbf{COH} & \textbf{CON} & \textbf{FC} & \textbf{SS} \\ \midrule
\textsc{gpt-4} & 1.14 & 1.64 & 2.00 & 1.29 & 0.86 \\
\textsc{Qwen2.5-72B-Instruct} & 1.11 & 1.57 & 1.71 & 1.29 & 0.86 \\
\textsc{Mistral-Large-Instruct-2407} & 1.03 & 1.36 & 2.00 & 1.14 & 0.86 \\
\textsc{gemma-2-27b-it} & 0.91 & 1.21 & 2.00 & 1.00 & 0.71 \\
\textsc{Meta-Llama-3.1-70B-Instruct} & 0.61 & 0.43 & 1.00 & 0.79 & 0.57 \\
\textsc{gpt-4o} & 0.54 & 0.57 & 1.86 & 0.57 & 0.43 \\
\textsc{Phi-3.5-MoE-instruct} & 0.44 & 0.57 & 1.86 & 0.43 & 0.29 \\
\textsc{llama38bGenZ\_Vikas-Merged} & 0.33 & 0.14 & 1.50 & 0.36 & 0.29 \\
\textsc{AryaBhatta-GemmaOrca-Merged} & 0.29 & 0.29 & 0.93 & 0.29 & 0.29 \\
\textsc{AryaBhatta-GemmaUltra-Merged} & 0.26 & 0.29 & 1.71 & 0.21 & 0.14 \\
\textsc{Indic-gemma-7b-finetuned-sft-Navarasa-2.0} & 0.19 & 0.29 & 0.57 & 0.21 & 0.07 \\
\textsc{telugu-llama-7b-instruct-v0.1} & 0.09 & 0.00 & 1.71 & 0.00 & 0.00 \\
\textsc{Telugu-Llama2-7B-v0-Instruct} & 0.00 & 0.00 & 0.00 & 0.00 & 0.00 \\ \bottomrule
\end{tabular}
\caption{Metric-wise scores for Telugu}
\label{tab:tel-scores}
\end{table*}
